# Supplementary material for: Bottlenecks in quantum channels and finite temperature phases of matter
Source: arXiv:2412.09598 source file (2026-10-16)
Supplement: Supplementary file 2 [file preamble_suppl.tex]

\usepackage[utf8]{inputenc}
\usepackage{amsmath}
\usepackage{amsthm}
\usepackage{enumitem}
\usepackage{amssymb}
\usepackage{wasysym}
\usepackage{oplotsymbl}
\usepackage{bm} %
\usepackage{dsfont} %
\usepackage{mathrsfs} %
\usepackage{physics}
\usepackage{mathtools}

\usepackage{xcolor}
\usepackage{framed}
\definecolor{darkblue}{rgb}{0,0,.65}
\definecolor{darkgreen}{rgb}{0.28,0.41,0.19}
\definecolor{nicegreen}{rgb}{0.28,0.85,0.19}




\usepackage[colorlinks=true,linkcolor=blue,allcolors=blue]{hyperref}
\usepackage[capitalize,nameinlink]{cleveref}

\def\figureautorefname{Fig.}
\def\equationautorefname~#1\null{Eq. (#1)\null}
\def\sectionautorefname{Sec.}
\newcommand{\appref}[1]{\hyperref[#1]{App.~\ref*{#1}}}

\renewcommand\vec{\bm}

\DeclareMathOperator\arctanh{arctanh}
\DeclareMathOperator\supp{supp}
\DeclareMathOperator\linspan{span}
\DeclareMathOperator\dist{dist}

\DeclarePairedDelimiter\ceil{\lceil}{\rceil}
\DeclarePairedDelimiter\floor{\lfloor}{\rfloor}

\newcommand{\hilbert}{\ensuremath{\mathscr{H}}}
\newcommand{\id}{\ensuremath{\mathds{1}}}
\newcommand{\muG}{\ensuremath{\mu_{\rm G}}}
\newcommand{\pG}{\ensuremath{p_{\rm G}}}
\newcommand{\rhoG}{\ensuremath{\hat \rho_{\rm G}}}
\newcommand{\rhoV}{\ensuremath{\hat \rho_{\mathcal{V}}}}
\newcommand{\rhoGV}{\ensuremath{\hat \rho_{G,\mathcal{V}}}}
\newcommand{\Sconf}{\ensuremath{S_{\rm conf}}}
\newcommand{\sconf}{\ensuremath{s_{\rm conf}}}
\newcommand{\Hcheck}{\ensuremath{H}}
\newcommand{\hamil}{\ensuremath{\hat{\mathcal H}}}
\newcommand{\reduced}{\ensuremath{\vert_{\rm red}}}
\newcommand{\indicator}{\ensuremath{\id}}

\newcommand{\wbit}{\ensuremath{w_{\rm bit}}}
\newcommand{\wcheck}{\ensuremath{w_{\rm check}}}

\newcommand{\muGTr}[1]{\ensuremath{\mu_{\rm G}^{\rm #1}}}
\newcommand{\maxConn}{\ensuremath{{\rm MaxConn}}}



\newtheorem{prototheorem}{Theorem}[section]
\newtheorem{protodef}[prototheorem]{Definition}
\newtheorem{conv}[prototheorem]{Convention}
\newtheorem{remark}[prototheorem]{Remark}
\newtheorem{protolemma}[prototheorem]{Lemma}
\newtheorem{cor}[prototheorem]{Corollary}
\newtheorem{proposition}[prototheorem]{Proposition}
\newtheorem{assume}[prototheorem]{Assumption}
\newtheorem{fact}[prototheorem]{Fact}
\newtheorem{claim}[prototheorem]{Claim}
\newtheorem{example}[prototheorem]{Example}
\newtheorem{protoconjecture}[prototheorem]{Conjecture}
\newtheorem{corollary}[prototheorem]{Corollary}
\newtheorem{task}[prototheorem]{Task}


\newenvironment{theorem}{\colorlet{shadecolor}{gray!15}\begin{shaded}\begin{prototheorem}}
{\end{prototheorem}\end{shaded}}

\newenvironment{lemma}{\colorlet{shadecolor}{gray!15}\begin{shaded}\begin{protolemma}}
{\end{protolemma}\end{shaded}}

\newenvironment{definition}{\colorlet{shadecolor}{gray!15}\begin{shaded}\begin{protodef}}
{\end{protodef}\end{shaded}}

\newenvironment{conjecture}{\colorlet{shadecolor}{gray!15}\begin{shaded}\begin{protoconjecture}}
{\end{protoconjecture}\end{shaded}}
